# Supplementary material for: Bayesian Copula Density Estimation Using Bernstein Yett-Uniform Priors
Source: arXiv:2405.04475 ancillary file (2024-05-07)
Supplement: Supplementary file 1 [file BYUP_arXiv_supplementary.pdf]

# **Supplementary Material for**

## **Bayesian Copula Density Estimation Using Bernstein**

### **Yett-Uniform Priors**

NICOLÁS KUSCHINSKI, RICHARD WARR AND ALEJANDRO JARA

May 7, 2024

---

<sup>1</sup>Nicolás Kuschinski is a Postdoctoral Researcher at the Department of Statistics, Pontificia Universidad Católica de Chile and the Center for the Discovery of Structures in Complex Data, Casilla 306, Correo 22, Santiago, Chile (E-mail: nicolas.kuschinski@mat.uc.cl). Richard Warr is an Associate Professor, Department of Statistics, Brigham Young University, Provo, UT 84602, USA (warr@stat.byu.edu). Alejandro Jara is an Associate Professor, Department of Statistics, Pontificia Universidad Católica de Chile and Center for the Discovery of Structures in Complex Data Casilla 306, Correo 22, Santiago, Chile (E-mail: atjara@uc.cl).

# 1 Proof of Theorem 1

We consider first the case where  $G$  is the restriction of the CDF of an absolutely continuous probability measure defined on  $[0, 1]^d$  and with uniform marginals. In Theorem 1, Sancetta and Satchell (2004) provided sufficient conditions on a general function  $G$  for its multivariate Bernstein polynomial to be a copula function. We show that if  $G$  is the restriction of the CDF of an absolutely continuous probability measure defined on  $[0, 1]^d$  and with uniform marginals, then those conditions are fulfilled and, hence,  $B_{\mathbf{k}, G}(z)$  is also a copula function. In our notation, the sufficient conditions derived by Sancetta and Satchell (2004) are given by

- (i)  $\sum_{l_1 \in \{0,1\}} \cdots \sum_{l_d \in \{0,1\}} (-1)^{l_1 + \cdots + l_d} G\left(\frac{\nu_1 + l_1}{k_1}, \dots, \frac{\nu_d + l_d}{k_d}\right) \geq 0$ , for all  $\nu_j \in \{1, \dots, k_j - 1\}$  and  $j = 1, \dots, d$ , and

$$\min\left(0, \frac{\nu_1}{k_1} + \cdots + \frac{\nu_d}{k_d} - (d-1)\right) \leq G\left(\frac{\nu_1}{k_1}, \dots, \frac{\nu_d}{k_d}\right) \leq \min\left(\frac{\nu_1}{k_1}, \dots, \frac{\nu_d}{k_d}\right),$$

- (ii)  $\lim_{\nu_j \rightarrow 0} G\left(\frac{\nu_1}{k_1}, \dots, \frac{\nu_d}{k_d}\right) = 0$ , for all  $\nu_j \in \{0, \dots, k_j\}$  and  $j = 1, \dots, d$ , and

- (iii)  $G\left(\frac{k_1}{k_1}, \dots, \frac{k_{j-1}}{k_{j-1}}, \frac{\nu_j}{k_j}, \frac{k_{j+1}}{k_{j+1}}, \dots, \frac{k_d}{k_d}\right) = \frac{\nu_j}{k_j}$  for all  $j = 1, \dots, d$ .

Since  $G$  is the restriction of the CDF of an absolutely continuous probability measure defined on  $[0, 1]^d$ , then

$$G(0, \dots, 0) = 0,$$

$$G(x_1, \dots, x_{i-1}, 0, x_{i+1}, \dots, x_d) = 0,$$

for all  $i = 1, \dots, d$ , and  $x_1, \dots, x_{i-1}, x_{i+1}, \dots, x_d \in [0, 1)$ , and

$$W_{\nu_1, \dots, \nu_d} = G\left(\left(\frac{\nu_1 - 1}{k_1}, \frac{\nu_1}{k_1}\right] \times \cdots \times \left(\frac{\nu_d - 1}{k_d}, \frac{\nu_d}{k_d}\right]\right) \geq 0,$$

for all  $\nu_j \in \{1, \dots, k_j\}$  and  $j = 1, \dots, d$ . Furthermore, since  $G$  is a copula function, it also satisfies the Boole-Fréchet bounds (Boole, 1854). Thus, condition (i) is satisfied.

Since  $G$  is the restriction of the CDF of an absolutely continuous probability measure defined on  $[0, 1]^d$  and with uniform marginals, then  $G(1, \dots, 1, 0, 1, \dots, 1)$  is the cumulative probability of a uniform distribution at 0, which is 0. We note that since  $G$  is the restriction of a CDF, then

$$G(0, \dots, 0, 0, 0, \dots, 0) \leq G(x_1, \dots, x_{i-1}, 0, x_{i+1}, \dots, x_d) \leq G(1, \dots, 1, 0, 1, \dots, 1),$$

for all  $x_i \in (0, 1)$ . Also,  $G$  is continuous. Thus  $G$  also meets condition (ii).

Finally, since  $G$  is the restriction of the CDF of a probability measure defined on  $[0, 1]^d$  and with uniform marginals, then  $G(1, \dots, 1, \frac{\nu_i}{k_i}, 1, \dots, 1)$  is the cumulative probability of a uniform distribution at  $\frac{\nu_i}{k_i}$ . Now, since  $0 \leq \nu_i \leq k_i$ , it follows that  $0 \leq \frac{\nu_i}{k_i} \leq 1$  and this value is  $\frac{\nu_i}{k_i}$ . Thus,  $G$  also meets condition (iii), which completes the proof that  $B_{\mathbf{k}, G}$  is a copula function when  $G$  is the restriction of the CDF of an absolutely continuous probability measure defined on

$[0, 1]^d$  and with uniform marginals.

Now we provide the proof for the discrete case. Specifically, assume that  $G$  is the restriction of the CDF of a discrete probability measure defined on  $(0, 1]^d$ , with uniform marginals, and with  $p_i$  support points,  $i = 1, \dots, d$ . We assume that the number of support points are such that  $\frac{p_i}{k_i}$  is an integer for all  $i \in \{1, \dots, d\}$ , for a given finite  $\mathbf{k} \in \mathbb{N}^d$ . Let  $\mathbf{p} = (p_1, \dots, p_d)$  and set

$$\rho^{\mathbf{p}} = \{0/p_1, 1/p_1, 2/p_1, \dots, p_1/p_1\} \times \dots \times \{0/p_d, 1/p_d, 2/p_d, \dots, p_d/p_d\},$$

and

$$\rho^{\mathbf{k}} = \{0/k_1, 1/k_1, 2/k_1, \dots, k_1/k_1\} \times \dots \times \{0/k_d, 1/k_d, 2/k_d, \dots, k_d/k_d\}.$$

Let  $\nu^{\rho^{\mathbf{k}}}$  be the collection of sets formed by  $\rho^{\mathbf{k}}$ , of the form

$$\left( \frac{l_1 - 1}{k_1}, \frac{l_1}{k_1} \right] \times \dots \times \left( \frac{l_d - 1}{k_d}, \frac{l_d}{k_d} \right],$$

where  $l_j \in \{1, \dots, k_j\}$ , which are indexed by their upper right (or higher dimensional equivalent). Now, let  $G_{\mathbf{p}}$  be the restriction of the CDF of the  $\rho^{\mathbf{p}}$ -uniform version of of the probability measure for which  $G$  is the restriction of the CDF to the unit hyper-cube (we refer the reader to Section 2.2 in the main paper for its definition). Notice that, by construction,  $G_{\mathbf{p}}$  is the restriction of the CDF of a yett-uniform copula of degree  $\mathbf{p}$  (we refer the reader to Section 2.2 in the main paper for its definition), which is an absolutely continuous probability measure. Furthermore, for every set  $A \in \nu^{\rho^{\mathbf{p}}}$ ,  $G_{\mathbf{p}}(A) = G(A)$ , which implies that  $B_{\mathbf{k}, G} = B_{\mathbf{k}, G_{\mathbf{p}}}$ . Now, since  $G_{\mathbf{p}}$  is an continuous probability distribution with uniform marginals, it follows from the first part of the current proof, that  $B_{\mathbf{k}, G_{\mathbf{p}}}$  is also a copula function and, therefore, the same can be said for  $B_{\mathbf{k}, G}$ .

Finally, since  $G(\mathbf{z}) = 0$  for  $\mathbf{z} \in \{\mathbf{y} \in [0, 1]^d : y_l > 0, l = 1, \dots, d\}^C$  in both cases, which ensures that  $B_{\mathbf{k}, G}$  is the restriction of the CDF of a probability measure that has a density w.r.t. Lebesgue measure (see, e.g., Barrientos et al., 2015), the expression for a density of  $B_{\mathbf{k}, G}$  can be easily found simply by differentiating  $B_{\mathbf{k}, G}$  in either of the cases.

□

## 2 Proof of Theorem 2

The proof follows the same arguments of the proof of Theorem 1 in Barrientos et al. (2015). By the multivariate version of the mean value theorem proposed by Ash (2008), there exists a real vector  $\mathbf{c}_{j_1, \dots, j_d}^{\mathbf{k}} \in \left(\frac{j_1-1}{k_1}, \frac{j_1}{k_1}\right] \times \dots \times \left(\frac{j_d-1}{k_d}, \frac{j_d}{k_d}\right]$  such that,

$$\sum_{i=0}^d \sum_{\{\mathbf{e} \in \{0,1\}^d: |\mathbf{e}|=i\}} (-1)^i G\left(\frac{j_1-e_1}{k_d}, \dots, \frac{j_d-e_d}{k_d}\right) = \frac{g(\mathbf{c}_{j_1, \dots, j_d}^{\mathbf{k}})}{\prod_{i=1}^d k_i},$$

for every  $(j_1, \dots, j_d) \in \mathcal{H}_{\mathbf{k},d}^0$ , where  $\mathcal{H}_{\mathbf{k},d}^0 = \{1, \dots, k_1\} \times \dots \times \{1, \dots, k_d\}$ . Therefore,

$$\begin{aligned} b_{\mathbf{k},G}(\mathbf{y}) &= \sum_{\mathbf{j} \in \mathcal{H}_{\mathbf{k},d}^0} G\left(\left(\frac{j_1-1}{k_1}, \frac{j_1}{k_1}\right] \times \dots \times \left(\frac{j_d-1}{k_d}, \frac{j_d}{k_d}\right]\right) \prod_{i=1}^d \beta(y_i | \alpha(\mathbf{k}, \mathbf{j})), \\ &= \sum_{\mathbf{j} \in \mathcal{H}_{\mathbf{k},d}^0} \frac{g(\mathbf{c}_{j_1, \dots, j_d}^{\mathbf{k}})}{\prod_{i=1}^d k_i} \prod_{i=1}^d \beta(y_i | \alpha(\mathbf{k}, \mathbf{j})), \\ &= C(\mathbf{k}, d) \sum_{\mathbf{j} \in \mathcal{J}_d^{\mathbf{k}-1}} g(\mathbf{c}_{j_1+1, \dots, j_d+1}^{\mathbf{k}}) \prod_{i=1}^d \text{Binom}(j_i | k_i - 1, y_i), \end{aligned}$$

where  $\mathcal{J}_d^{\mathbf{k}-1} = \{0, \dots, k_1 - 1\} \times \dots \times \{0, \dots, k_d - 1\}$  and  $C(\mathbf{k}, d) = \prod_{i=1}^d \frac{k_i + d - i + 1}{k_i}$ .

Recall that  $k = \min\{k_1, \dots, k_d\}$ . Now, since  $g$  is continuous, then for every  $\epsilon > 0$  there exists a positive integer  $k_0$  such that if  $k \geq k_0$  and  $\mathbf{a}, \mathbf{b} \in \left(\frac{j_1}{k-d}, \frac{j_1+1}{k-d}\right] \times \dots \times \left(\frac{j_d}{k-d}, \frac{j_d+1}{k-d}\right]$ ,  $(j_1, \dots, j_d) \in \mathcal{J}_d^{\mathbf{k}-1} = \{0, \dots, k-1\}^d$ , then  $|g(\mathbf{a}) - g(\mathbf{b})| < \epsilon$ . Thus, for every  $(j_1, \dots, j_d) \in \mathcal{J}_d^{\mathbf{k}-1}$  and  $k \geq k_0$ , it follows that

$$\left| g\left(\frac{j_1}{k}, \dots, \frac{j_d}{k}\right) - g(\mathbf{c}_{j_1+1, \dots, j_d+1}^{\mathbf{k}}) \right| < \epsilon,$$

and, therefore,

$$\begin{aligned} &\sup_{\mathbf{y} \in [0,1]^d} |b_{\mathbf{k},G}(\mathbf{y}) - g(\mathbf{y})| \\ &\leq C(k, d) \left| \sup_{\mathbf{y} \in [0,1]^d} \sum_{\mathbf{j} \in \mathcal{J}_d^{\mathbf{k}-1}} g(\mathbf{c}_{j_1+1, \dots, j_d+1}^{\mathbf{k}}) - g\left(\frac{j_1}{k}, \dots, \frac{j_d}{k}\right) \text{Multinom}(\mathbf{j} | k-1, \mathbf{y}) \right| \\ &\quad + \sup_{\mathbf{y} \in [0,1]^d} \left| g(\mathbf{y}) - C(k, d) \sum_{\mathbf{j} \in \mathcal{J}_d^{\mathbf{k}-1}} g\left(\frac{j_1}{k}, \dots, \frac{j_d}{k}\right) \text{Multinom}(\mathbf{j} | k-1, \mathbf{y}) \right|, \\ &\leq C(k, d)\epsilon + \sup_{\mathbf{y} \in [0,1]^d} |g(\mathbf{y}) - B_{k-d,g}(\mathbf{y})| k, \end{aligned}$$

where  $C(k, d) = \prod_{i=1}^d \frac{k+d-i+1}{k}$ . The proof of the uniform approximation is completed by noticing that  $C(k, d)$  and  $B_{k-d,g}$  converge to 1 and  $g$ , respectively, as  $k \rightarrow \infty$ .

Let  $\mathbf{z}_j = (z_{j,1}, \dots, z_{j,d+1}) \stackrel{i.i.d.}{\sim} \text{Multinomial}(1, \boldsymbol{\pi})$ , where  $\boldsymbol{\pi} = \left(\mathbf{y}, 1 - \sum_{l=1}^d y_l\right)$ . Set  $\mathbf{S}_{\mathbf{k}} = \sum \mathbf{z}_j$  and  $\mathbf{W}_{\mathbf{k}} = (S_{\mathbf{k},1}, \dots, S_{\mathbf{k},d})$ . By the multivariate version of the mean value theorem proposed by Ash (2008), it is possible to

ensure the existence of a  $(0, 1)$ -value random vector  $\mathbf{c}_{\mathbf{W}_k}$  such that,

$$G\left(\left(\frac{S_{k,1}}{k_1}, \frac{S_{k,1}+1}{k_1}\right] \times \dots \times \left(\frac{S_{k,d}}{k_d}, \frac{S_{k,d}+1}{k_d}\right]\right) = \frac{g\left(\frac{\mathbf{W}_k + \mathbf{c}_{\mathbf{W}_k}}{\mathbf{k}}\right)}{\prod_{i=1}^d k_i},$$

where we use  $\frac{\mathbf{W}_k + \mathbf{c}_{\mathbf{W}_k}}{\mathbf{k}}$  to denote the vector obtained by dividing  $\mathbf{W}_k + \mathbf{c}_{\mathbf{W}_k}$  by  $\mathbf{k}$  element-wise.

Thus, it follows that

$$b_{k,G}(\mathbf{y}) = \prod_{i=1}^d \frac{\sum_{v_s=1}^{k_i} v_s! (k_i - v_s + 1)!}{k_i + 1!} E_{\mathbf{S}_k} \left[ g\left(\frac{\mathbf{W}_k + \mathbf{c}_{\mathbf{W}_k}}{\mathbf{k}}\right) \right]. \quad (1)$$

Therefore, for  $\alpha \in (0, 1]$ ,

$$\begin{aligned} \|g - b_{k,G}\|_\infty &\leq \sup_{\mathbf{y} \in [0,1]^d} \left| g(\mathbf{y}) - E_{\mathbf{S}_k} \left[ g\left(\frac{\mathbf{W}_k + \mathbf{c}_{\mathbf{W}_k}}{k}\right) \right] \right| \\ &\quad + \sup_{\mathbf{y} \in [0,1]^d} \left| E_{\mathbf{S}_k} \left[ g\left(\frac{\mathbf{W}_k + \mathbf{c}_{\mathbf{W}_k}}{k}\right) \right] - \frac{(k+d-1)!}{(k-1)!k^d} E_{\mathbf{S}_k} \left[ g\left(\frac{\mathbf{W}_k + \mathbf{c}_{\mathbf{W}_k}}{k}\right) \right] \right|, \\ &\leq L_\alpha(g) \sup_{\mathbf{y} \in [0,1]^d} E_{\mathbf{S}_k} \left[ \sum_{j=1}^d \left( y_j - \frac{W_{k,j} + c_{W_{k,j}}}{k} \right)^2 \right]^{\alpha/2} + \left| 1 - \frac{(k+d-1)!}{(k-1)!k^d} \right| \|g\|_\infty. \end{aligned}$$

Now, since

$$\begin{aligned} E_{\mathbf{S}_k} \left[ \sum_{j=1}^d \left( y_j - \frac{W_{k,j} + c_{W_{k,j}}}{k} \right)^2 \right] &= k^{-2} E_{\mathbf{S}_k} \left[ \sum_{j=1}^d (k_j y_j - W_{k,j})^2 - 2(k_j y_j - W_{k,j}) c_{W_{k,j}} + c_{W_{k,j}}^2 \right], \\ &\leq k^{-2} \sum_{j=1}^d (\text{Var}[W_{k,j}] + 1) \leq \sum_{j=1}^d \frac{y_j(1-y_j)}{k} + \frac{d}{k^2}, \end{aligned}$$

it follows that,

$$\|g - b_{k,G}\|_\infty \leq d L_\alpha(g) \left( \frac{1}{2k} + \frac{1}{k^2} \right)^{\alpha/2} + \left| 1 - \frac{(k+d-1)!}{(k-1)!k^d} \right| \|g\|_\infty.$$

Now let  $\alpha \in (1, 2]$ . By using the triangle inequality, it follows that

$$\begin{aligned} \|g - b_{k,G}\|_\infty &\leq \sup_{\mathbf{y} \in [0,1]^d} \left| g(\mathbf{y}) - g\left(\frac{k-1}{k}\mathbf{y}\right) \right| + \\ &\quad \sup_{\mathbf{y} \in [0,1]^d} \left| g\left(\frac{k-1}{k}\mathbf{y}\right) - k^d E_{\mathbf{S}_k} \left[ G\left(\left(\frac{W_{k,1}}{k}, \frac{W_{k,1}+1}{k}\right] \times \dots \times \left(\frac{W_{k,d}}{k}, \frac{W_{k,d}+1}{k}\right]\right) \right] \right| + \\ &\quad \sup_{\mathbf{y} \in [0,1]^d} \left| k^d E_{\mathbf{S}_k} \left[ G\left(\left(\frac{W_{k,1}}{k}, \frac{W_{k,1}+1}{k}\right] \times \dots \times \left(\frac{W_{k,d}}{k}, \frac{W_{k,d}+1}{k}\right]\right) \right] \right. \\ &\quad \left. - \frac{(k+d-1)!}{(k-1)!} E_{\mathbf{S}_k} \left[ G\left(\left(\frac{W_{k,1}}{k}, \frac{W_{k,1}+1}{k}\right] \times \dots \times \left(\frac{W_{k,d}}{k}, \frac{W_{k,d}+1}{k}\right]\right) \right] \right|. \end{aligned}$$

Since every function with bounded partial derivatives is a Lipchitz function, it is straightforward to see that

$$\sup_{\mathbf{y} \in [0,1]^d} \left| g(\mathbf{y}) - g\left(\frac{k-1}{k}\mathbf{y}\right) \right| \leq \frac{d}{k} \max_{l \in \{1, \dots, d\}} \|D_1^{y_l} g\|_\infty. \quad (2)$$

Now, by the sequential application of Taylor's Theorem with integral remainder, it follows that

$$\begin{aligned}
& k^d E_{\mathbf{S}_k} \left[ G \left( \left( \frac{W_{k,1}}{k}, \frac{W_{k,1}+1}{k} \right) \times \dots \times \left( \frac{W_{k,d}}{k}, \frac{W_{k,d}+1}{k} \right) \right) \right] = \\
& E_{\mathbf{S}_k} \left[ D_1^{y_d} \dots D_1^{y_1} G \left( \frac{W_{k,1}}{k}, \dots, \frac{W_{k,d}}{k} \right) \right] + \sum_{l=1}^d \frac{1}{k^l} \sum_{(j_1, \dots, j_d) \in \mathcal{D}_l^d} E_{\mathbf{S}_k} \left[ \int_0^1 \dots \int_0^1 \right. \\
& \left. D_{j_d}^{y_d} \dots D_{j_1}^{y_1} G \left( \frac{W_{k,1} + s_1(j_1-1)}{k}, \dots, \frac{W_{k,d} + s_d(j_d-1)}{k} \right) \prod_{i=1}^d (1 - s_i(j_i-1)) ds_1 \dots ds_d \right]. \quad (3)
\end{aligned}$$

On the other hand, the mean value Theorem for functions of several variables given in Section 6.2 of Courant (1950), implies that there exists a constant  $\gamma \in (0, 1)$  such that

$$\begin{aligned}
& \left| g(\mathbf{y} + \mathbf{h}) - g(\mathbf{y}) - \sum_{l=1}^d h_l D_1^{y_l} g(y_1, \dots, y_d) \right| \\
& \leq \sum_{l=1}^d |h_l| |D_1^{y_l} g(y_1 + \gamma h_1, \dots, y_d + \gamma h_d) - D_1^{y_l} g(y_1, \dots, y_d)|, \\
& \leq \sqrt{d} \max_{l \in \{1, \dots, d\}} L_\alpha(D_1^{y_l} g) \left[ \sum_{l=1}^d |h_l| \right]^\alpha,
\end{aligned}$$

and therefore,

$$\begin{aligned}
& \left| g\left(\frac{\mathbf{W}_k}{k}\right) - g\left(\frac{k-1}{k}\mathbf{y}\right) - \sum_{l=1}^d \left(\frac{W_{k,l}}{k} - \frac{k-1}{k}y_l\right) D_1^{y_l} g\left(\frac{k-1}{k}\mathbf{y}\right) \right| \\
& \leq \sqrt{d} \max_{l \in \{1, \dots, d\}} L_\alpha(D_1^{y_l} g) \left[ \sum_{l=1}^d \left| \frac{W_{k,l}}{k} - \frac{k-1}{k}y_l \right| \right]^\alpha. \quad (4)
\end{aligned}$$

Thus, by combining (3) and (4), it follows that

$$\begin{aligned}
& \sup_{\mathbf{y} \in [0,1]^d} \left| g\left(\frac{k-1}{k}\mathbf{y}\right) - k^d E_{\mathbf{S}_k} \left[ G \left( \left( \frac{W_{k,1}}{k}, \frac{W_{k,1}+1}{k} \right) \times \dots \times \left( \frac{W_{k,d}}{k}, \frac{W_{k,d}+1}{k} \right) \right) \right] \right| \\
& \leq \sup_{\mathbf{y} \in [0,1]^d} \left| g\left(\frac{k-1}{k}\mathbf{y}\right) - E_{\mathbf{S}_k} \left[ g\left(\frac{W_{k,1}}{k}, \dots, \frac{W_{k,d}}{k}\right) \right] \right| \\
& \quad + \sum_{l=1}^d \frac{1}{k^l} \binom{d}{l} \max_{(j_1, \dots, j_d) \in \mathcal{D}_l^d} \|D_{j_d}^{y_d} \dots D_{j_1}^{y_1} G\|_\infty. \quad (5)
\end{aligned}$$

In addition, an application of Jensen's inequality implies that

$$\begin{aligned}
& \sup_{\mathbf{y} \in [0,1]^d} \left| g\left(\frac{k-1}{k}\mathbf{y}\right) - E_{\mathbf{S}_k} \left[ g\left(\frac{W_{\mathbf{k},1}}{k}, \dots, \frac{W_{\mathbf{k},d}}{k}\right) \right] \right| \\
& \leq E_{\mathbf{S}_k} \left[ \left| g\left(\frac{\mathbf{W}_k}{k}\right) - g\left(\frac{k-1}{k}\mathbf{y}\right) - \sum_{l=1}^d \left(\frac{W_{\mathbf{k},l}}{k} - \frac{k-1}{k}y_l\right) D_1^{y_l} g\left(\frac{k-1}{k}\mathbf{y}\right) \right| \right], \\
& \leq \sqrt{d} \max_{l \in \{1, \dots, d\}} L_\alpha(D_1^{y_l} g) \left( E_{\mathbf{S}_k} \left[ \sum_{l=1}^d \left| \frac{W_{\mathbf{k},l}}{k} - \frac{k-1}{k}y_l \right| \right]^2 \right)^{\alpha/2}, \\
& = \sqrt{d} \max_{l \in \{1, \dots, d\}} L_\alpha(D_1^{y_l} g) \left( Var \left[ \sum_{l=1}^d \left| \frac{W_{\mathbf{k},l}}{k} - \frac{k-1}{k}y_l \right| \right] + \left( E_{\mathbf{S}_k} \left[ \sum_{l=1}^d \left| \frac{W_{\mathbf{k},l}}{k} - \frac{k-1}{k}y_l \right| \right] \right)^2 \right)^{\alpha/2}.
\end{aligned}$$

Since

$$E_{\mathbf{S}_k} \left[ \left| \frac{W_{\mathbf{k},l}}{k} - \frac{k-1}{k}y_l \right| \right] = E_{\mathbf{S}_k} \left[ \left| \frac{W_{\mathbf{k},l}}{k} - \frac{k-1}{k}y_l \right|^2 \right]^{1/2} \leq (k^{-2} Var[W_{\mathbf{k},l}])^{1/2} \leq \frac{1}{2k^{1/2}},$$

and

$$\begin{aligned}
& Var \left[ \sum_{l=1}^d \left| \frac{W_{\mathbf{k},l}}{k} - \frac{k-1}{k}y_l \right| \right] \\
& \leq \sum_{l=1}^d Var \left[ \left| \frac{W_{\mathbf{k},l}}{k} - \frac{k-1}{k}y_l \right| \right] + \sum_{l_1 \neq l_2} \left( Var \left[ \left| \frac{W_{\mathbf{k},l_1}}{k} - \frac{k-1}{k}y_{l_1} \right| \right] Var \left[ \left| \frac{W_{\mathbf{k},l_2}}{k} - \frac{k-1}{k}y_{l_2} \right| \right] \right)^{1/2}, \\
& \leq \frac{d}{4k} + \frac{d(d+1)}{4k},
\end{aligned}$$

it follows that

$$\sup_{\mathbf{y} \in [0,1]^d} \left| g\left(\frac{k-1}{k}\mathbf{y}\right) - E_{\mathbf{S}_k} \left[ g\left(\frac{W_{\mathbf{k},1}}{k}, \dots, \frac{W_{\mathbf{k},d}}{k}\right) \right] \right| \leq \sqrt{d} \max_{l \in \{1, \dots, d\}} L_\alpha(D_1^{y_l} g) \left( \frac{d(1+d)}{2k} \right)^{\alpha/2}. \quad (6)$$

Finally, for the third term, one has by (1) that

$$\begin{aligned}
& \sup_{\mathbf{y} \in [0,1]^d} \left| k^d E_{\mathbf{S}_k} \left[ G \left( \left( \frac{W_{\mathbf{k},1}}{k}, \frac{W_{\mathbf{k},1}+1}{k} \right) \times \dots \times \left( \frac{W_{\mathbf{k},d}}{k}, \frac{W_{\mathbf{k},d}+1}{k} \right) \right) \right] \right. \\
& \quad \left. - \frac{(k+d-1)!}{(k-1)!} E_{\mathbf{S}_k} \left[ G \left( \left( \frac{W_{\mathbf{k},1}}{k}, \frac{W_{\mathbf{k},1}+1}{k} \right) \times \dots \times \left( \frac{W_{\mathbf{k},d}}{k}, \frac{W_{\mathbf{k},d}+1}{k} \right) \right) \right] \right| \\
& \leq d^2(d-1)!k^{d-1} E_{\mathbf{S}_k} \left[ G \left( \left( \frac{W_{\mathbf{k},1}}{k}, \frac{W_{\mathbf{k},1}+1}{k} \right) \times \dots \times \left( \frac{W_{\mathbf{k},d}}{k}, \frac{W_{\mathbf{k},d}+1}{k} \right) \right) \right], \\
& \leq \frac{d^2(d-1)!}{k} \|g\|_\infty.
\end{aligned} \quad (7)$$

Putting together (2), (5), (6) and (7), completes the proof of the theorem.  $\square$

### 3 Proof of Proposition 1

Let  $C_1$  and  $C_2 \in \tilde{\mathcal{C}}_{d,\mathbf{k}}$  be two yett-uniform copulas of degree  $\mathbf{k}$ . Notice that if  $C_1$  and  $C_2$  have the same weights  $\{W_{\nu_1, \dots, \nu_d}\}$ , then  $C_1 = C_2$ . This is true because

$$W_{\nu_1, \dots, \nu_d} = C_1 \left( \left( \frac{\nu_1 - 1}{k_1}, \frac{\nu_1}{k_1} \right] \times \dots \times \left( \frac{\nu_d - 1}{k_d}, \frac{\nu_d}{k_d} \right] \right) = C_2 \left( \left( \frac{\nu_1 - 1}{k_1}, \frac{\nu_1}{k_1} \right] \times \dots \times \left( \frac{\nu_d - 1}{k_d}, \frac{\nu_d}{k_d} \right] \right),$$

and since  $C_1$  and  $C_2$  are yett-uniform then the densities of  $c_1(\mathbf{x}) = c_2(\mathbf{x})$  for all  $\mathbf{x}$  within a cell of the yett. Since the space  $[0, 1]^d$  is the union of the cells, then they match over the entire domain. This proves that the mapping is injective.

To prove that the mapping is surjective, let  $b_{\mathbf{k},G}(\mathbf{z}) = \sum_{\nu_1=1}^{k_1} \dots \sum_{\nu_d=1}^{k_d} W_{\nu_1, \dots, \nu_d} \prod_{j=1}^d \beta(z_j \mid \nu_j, k_j - \nu_j + 1)$  be an arbitrary Bernstein copula density, meaning it is density of the Bernstein polynomial corresponding to some absolutely continuous copula  $C$ . Then let  $C_{\rho^{\mathbf{k}}}$  be the  $\rho^{\mathbf{k}}$ -uniform distribution which assigns to each cell in  $\rho^{\mathbf{k}}$  the same probability assigned by  $C$ . We observe that in fact  $C_{\rho^{\mathbf{k}}}$  is a  $\rho^{\mathbf{k}}$ -uniform copula, and that  $B_{\mathbf{k},C}(\mathbf{z}) = B_{\mathbf{k},C_{\rho^{\mathbf{k}}}}(\mathbf{z})$ . Hence the mapping is surjective, which completes the proof.  $\square$

## 4 Proof of Theorem 3

Let  $\mathcal{A}$  be a nonempty open set in  $\mathcal{C}_d$ . Take a copula  $C^{(0)} \in \mathcal{A}$ . Now we observe that by the uniform approximation of Bernstein polynomials, there is a  $\mathbf{k} \in \mathbb{N}^d$  such that  $C^{(1)} = B_{\mathbf{k}, C^{(0)}} \in \mathcal{A}$ . It follows that there is an  $\epsilon > 0$ , such that  $\{C \in \mathcal{C}_d : \mathcal{H}^2(C^{(1)}, C) < \epsilon\} \subseteq \mathcal{A}$ , where  $\mathcal{H}^2$  is the squared Hellinger distance. Now, by Proposition 1, we know that there is therefore a unique  $\rho^{\mathbf{k}}$ -uniform copula  $D^{(1)}$  such that  $T_{[0,1]^d} \circ BP_{(\rho^{\mathbf{k}}, D^{(1)})} = C^{(1)}$ . Let  $\mathbf{W}^{(1)}$  be a vector containing the weights of  $D^{(1)}$ ,  $\{W_{\nu_1, \dots, \nu_d}^{(1)} : \nu_j \in \{1, \dots, k_j\}, j = 1, \dots, d\}$ , in some appropriate order.

We now observe that the density of  $C^{(1)}$  is  $c^{(1)}(\mathbf{z}) = \sum_{\nu_1=1}^{k_1} \cdots \sum_{\nu_d=1}^{k_d} W_{\nu_1, \dots, \nu_d}^{(1)} \prod_{j=1}^d \beta(z_j \mid \nu_j, k_j - \nu_j + 1)$ . Since this is a polynomial of fixed degree on a compact domain, there is a  $\epsilon_1 > 0$  such that if  $\mathbf{W}^{(*)}$  is another vector with  $\|\mathbf{W}^{(*)}, \mathbf{W}^{(1)}\| < \epsilon_1$ , then  $c^{(*)}(\mathbf{z}) = \sum_{\nu_1=1}^{k_1} \cdots \sum_{\nu_d=1}^{k_d} W_{\nu_1, \dots, \nu_d}^{(*)} \prod_{j=1}^d \beta(z_j \mid \nu_j, k_j - \nu_j + 1)$  has the property that  $\left(\sqrt{c^{(*)}(\mathbf{z})} - \sqrt{c^{(1)}(\mathbf{z})}\right)^2 < \epsilon$ , for all  $\mathbf{z} \in [0, 1]^d$ .

We note that in Lemma 1 of the Supplementary Material of Kuschinski and Jara (2023), it is proven that for grid-uniform copulas, which include yett-uniform copulas as a particular case, the mapping between a copula and its parameters is continuous in both the Hellinger and Kullback–Leibler sense. Hence, there is a Hellinger neighborhood  $\mathcal{B}_\delta \subset \mathcal{C}_d^*$  such that for any  $E$  in  $\mathcal{B}_\delta$ , the corresponding vector of weights of cells assigned by  $E$ ,  $\mathbf{W}^{(E)}$  has the property that  $\|\mathbf{W}^{(E)} - \mathbf{W}^{(1)}\| < \epsilon_1$ . Then, if  $D^{(2)} \in \mathcal{B}_\delta$  we write  $C^{(2)} = T_{[0,1]^d} \circ BP_{(\rho^{\mathbf{k}}, D^{(2)})}$  and

$$c^{(2)}(\mathbf{z}) = \sum_{\nu_1=1}^{k_1} \cdots \sum_{\nu_d=1}^{k_d} W_{\nu_1, \dots, \nu_d}^{(2)} \prod_{j=1}^d \beta(z_j \mid \nu_j, k_j - \nu_j + 1),$$

is the density of  $C^{(2)}$ . Thus, the squared Hellinger distance,  $\mathcal{H}^2$ , is given by

$$\begin{aligned} \mathcal{H}^2(C^{(2)}, C^{(1)}) &= \frac{1}{2} \int_{[0,1]^d} \left( \sqrt{c^{(2)}(\mathbf{z})} - \sqrt{c^{(1)}(\mathbf{z})} \right)^2 d\mathbf{z}, \\ &\leq \frac{1}{2} \int_{[0,1]^d} \epsilon d\mathbf{z}, \\ &= \frac{1}{2} \epsilon < \epsilon, \end{aligned}$$

so  $C^{(2)} \in \mathcal{A}$ . Hence  $\{T_{[0,1]^d} \circ BP_{(\rho^{\mathbf{k}}, G)} : G \in \mathcal{B}_\delta\} \subseteq \mathcal{A}$ , which completes the proof. □

## 5 Proof of Theorem 4

Let  $\mathcal{A}$  be a nonempty open Kullback–Leibler set in  $\mathcal{C}_d$ . Take a copula  $C^{(0)} \in \mathcal{A}$ . Now, since  $C^{(0)}$  is strictly positive, continuous, and has finite entropy, then we observe that by the uniform approximation of Bernstein polynomials, there is a  $\mathbf{k} \in \mathbb{N}^d$ , such that  $C^{(1)} = B_{\mathbf{k}, C^{(0)}} \in \mathcal{A}$ . Thus, there is an  $\epsilon > 0$  such that  $\{C \in \mathcal{C}_d : \mathcal{KL}(C^{(1)}, C) < \epsilon\} \subseteq \mathcal{A}$ , where  $\mathcal{KL}$  is the Kullback–Leibler divergence. Now, by Proposition 1, we know that there is a unique  $\rho^{\mathbf{k}}$ -uniform copula  $D^{(1)}$  such that  $T_{[0,1]^d} \circ BP_{(\rho^{\mathbf{k}}, D^{(1)})} = C^{(1)}$ .

We note that  $C^{(1)}$  has density  $c^{(1)}$ , which is continuous and strictly positive on a compact domain, so it has a maximum  $c_{\max}^{(1)} > 0$ . Let  $\mathbf{W}^{(1)}$  be a vector containing the weights of  $D^{(1)}$ ,  $\{W_{\nu_1, \dots, \nu_d}^{(1)} : \nu_j \in \{1, \dots, k_j\}, j = 1, \dots, d\}$ , in some appropriate order. Since  $c^{(1)}$  is a polynomial of fixed degree on a compact domain, there is an  $\epsilon_1 > 0$ , such that if  $\mathbf{W}^*$  is another vector with  $\|\mathbf{W}^*, \mathbf{W}^{(1)}\| < \epsilon_1$ . It follows that

$$c^*(\mathbf{z}) = \sum_{\nu_1=1}^{k_1} \cdots \sum_{\nu_d=1}^{k_d} W_{\nu_1, \dots, \nu_d}^* \prod_{j=1}^d \beta(z_j \mid \nu_j, k_j - \nu_j + 1),$$

is strictly positive and has the property that

$$\log \left( \frac{c^1(\mathbf{x})}{c^*(\mathbf{x})} \right) < \frac{\epsilon}{c_{\max}^{(1)}},$$

for all  $\mathbf{x} \in [0, 1]^d$ .

In Lemma 1 from Appendix I of the Supplementary Material of Kuschinski and Jara (2023), it is proven that for grid-uniform copulas, which include yett-uniform copulas as a special case, the mapping between a copula and its parameters is continuous in both the Hellinger and Kullback–Leibler sense. Therefore, there is a Kullback–Leibler neighborhood  $\mathcal{B}_\delta \subset \mathcal{C}_d^*$ , such that for any  $D^{(2)}$  in  $\mathcal{B}_\delta$ , the corresponding vector of weights of cells assigned by  $D^{(2)}$ ,  $\mathbf{W}^{(2)}$  has the property that  $\|\mathbf{W}^{(2)} - \mathbf{W}^{(1)}\| < \epsilon_1$ . Then, if  $D^{(2)} \in \mathcal{B}_\delta$  we write  $C^{(2)} = T_{[0,1]^d} \circ BP_{(\rho^{\mathbf{k}}, D^{(2)})}$ , and  $c^{(2)}(\mathbf{z})$  is the density of  $C^{(2)}$ . Now, it follows that

$$\begin{aligned} \mathcal{KL}^2(C^{(2)}, C^{(1)}) &= \int_{[0,1]^d} c^{(1)}(\mathbf{z}) \log \left( \frac{c^{(1)}(\mathbf{z})}{c^{(2)}(\mathbf{z})} \right) d\mathbf{z}, \\ &< \int_{[0,1]^d} c_{\max}^{(1)} \frac{\epsilon}{c_{\max}^{(1)}} d\mathbf{z}, \\ &= \epsilon, \end{aligned}$$

so  $C^{(2)} \in \mathcal{A}$ . Hence  $\{T_{[0,1]^d} \circ BP_{(\rho^{\mathbf{k}}, G)} : G \in \mathcal{B}_\delta\} \subseteq \mathcal{A}$ , which completes the proof.  $\square$

## 6 Proof of Theorem 5

Set  $M \in \mathcal{C}_d$  and  $\epsilon > 0$ . By the uniform continuity of the square root function, there is an  $\epsilon_1 > 0$ , such that if  $|a - b| < \epsilon_1$ , then  $|\sqrt{a} - \sqrt{b}| < \sqrt{\epsilon}$ . Consider the case when  $M$  has continuous density  $m$ . Then we know that  $b_{\mathbf{k}, M}$  converges to  $m$  uniformly as  $k_1, \dots, k_d \rightarrow \infty$ . Then, there is a positive integer  $\lambda$  such that, for all  $\mathbf{l} \in \mathbb{N}^d$  with  $l_i \geq \lambda$ ,  $i = 1, \dots, d$ , it follows that

$$|b_{\mathbf{l}, M}(\mathbf{x}) - m(\mathbf{x})| < \epsilon_1,$$

for all  $\mathbf{x} \in [0, 1]^d$ .

Now pick  $\mathbf{l}$  such that  $l_i > \lambda$ ,  $i = 1, \dots, d$  and  $p_{\mathbf{k}}(\mathbf{l}) > 0$ . It follows that the squared Hellinger distance between  $M$  and  $B_{\mathbf{l}, M}$  is given by

$$\begin{aligned} \mathcal{H}^2(M, B_{\mathbf{l}, M}) &= \frac{1}{2} \int_{[0, 1]^d} \left( \sqrt{m(\mathbf{z})} - \sqrt{b_{\mathbf{l}, M}(\mathbf{z})} \right)^2 d\mathbf{z}, \\ &\leq \frac{1}{2} \int_{[0, 1]^d} \sqrt{\epsilon}^2 d\mathbf{z}, \\ &= \frac{1}{2} \epsilon. \end{aligned}$$

Now consider the case if  $M$  does not admit a continuous density,  $m$ . Note that the set of the discontinuities in  $m$  has measure zero. It is, therefore, possible to partition  $[0, 1]^d$  into two regions  $R_1$  and  $R_2$ , where  $R_1$  is a compact region where  $m$  is continuous, and  $R_2$  is the complement of  $R_1$ . We observe that this partition can be done so that the measure of  $R_2$  is as small as needed. It follows that

$$\mathcal{H}^2(M, B_{\mathbf{l}, M}) = \frac{1}{2} \int_{R_1} \left( \sqrt{m(\mathbf{z})} - \sqrt{b_{\mathbf{l}, M}(\mathbf{z})} \right)^2 d\mathbf{z} + \frac{1}{2} \int_{R_2} \left( \sqrt{m(\mathbf{z})} - \sqrt{b_{\mathbf{l}, M}(\mathbf{z})} \right)^2 d\mathbf{z}.$$

The first summand can be made arbitrarily small by the argument above. Since  $R_2$  can be picked to have arbitrarily small measure, it can be picked so that  $\frac{1}{2} \int_{R_2} \left( \sqrt{m(\mathbf{z})} - \sqrt{b_{\mathbf{l}, M}(\mathbf{z})} \right)^2 d\mathbf{z} < \frac{\epsilon}{2}$ . Hence we can pick  $\mathbf{l}$  such that  $\mathcal{H}^2(m, B_{\mathbf{l}, M}) < \epsilon/2 + \epsilon/2 = \epsilon$  regardless of whether  $M$  has continuous density or not. By Proposition 1, there is a unique yett-uniform copula  $C^{(0)}$  such that  $T_{[0, 1]^d} \circ BP_{(\rho^{\mathbf{l}}, C^{(0)})} = B_{\mathbf{l}, M}$ . By Theorem 3, there is an open Hellinger neighborhood of  $C^{(0)}$ ,  $A_\epsilon^{C^{(0)}}$  such that if  $C \in \{T_{[0, 1]^d} \circ BP_{(\rho^{\mathbf{k}}, G)} : G \in A_\epsilon^{C^{(0)}}\}$ , then  $\mathcal{H}^2(C, B_{\mathbf{l}, M}) < \frac{\epsilon}{2}$ .

In Lemma 2 of the Supplementary Material of Kuschinski and Jara (2023), they showed that open sets in both the Hellinger and Kullback–Leibler sense have positive probability under the prior  $p(\cdot \mid \mathbf{k}, \alpha, G_0)$ , for any  $\mathbf{k} \in \mathbb{N}^d$ . Hence,

$$p(\{T_{[0, 1]^d} \circ BP_{(\rho^{\mathbf{k}}, G)} : G \in A_\epsilon^{C^{(0)}}\} \mid \mathbf{l}, \alpha, G_0) > 0.$$

Observe that  $\{T_{[0, 1]^d} \circ BP_{(\rho^{\mathbf{k}}, G)} : G \in A_\epsilon^{C^{(0)}}\} \subseteq A_\epsilon^M$  so

$$\Pi(A_\epsilon^M \mid \alpha, G_0, p_{\mathbf{k}}) \geq p(\{T_{[0, 1]^d} \circ BP_{(\rho^{\mathbf{k}}, G)} : G \in A_\epsilon^{C^{(0)}}\} \mid \mathbf{l}, \alpha, G_0) > 0,$$

which completes the proof. □

## 7 Proof of Theorem 6

Let  $M \in \tilde{\mathcal{C}}_d$  be arbitrary. From Theorem 2 we know that  $B_{\mathbf{k},M}$  converges to  $M$  uniformly as  $k_1, \dots, k_d \rightarrow \infty$ . Let  $\epsilon > 0$  be arbitrary. Since  $M$  has a strictly positive density  $m$  and  $[0, 1]^d$  is compact, then  $B_{\mathbf{k},M}$  also has a strictly positive density for every  $\mathbf{k}$ , and in fact, there is a lower bound  $\beta$ , such that  $0 < \beta < m(\mathbf{x})$  and  $0 < \beta < b_{\mathbf{k},M}(\mathbf{x})$  for all  $\mathbf{x} \in [0, 1]^d$ .

We now observe that since  $M$  is absolutely continuous, the set of discontinuities in  $m$  has measure 0. We will partition  $[0, 1]^d$  into three regions.  $R_1$  is a compact region where  $m$  is continuous.  $R_2$  is a region made of balls of radius at most  $\gamma$  (from condition (ii)), and where each ball has a point  $\mathbf{y}$  where  $m(\mathbf{y}) > B$  (from condition (ii)). Lastly, let  $R_3$  be the remainder of  $[0, 1]^d$ . We observe that it is possible to select these regions such that  $R_3$  has arbitrarily small measure.

We observe now that the KL divergence

$$\begin{aligned} \mathcal{KL}(M, B_{\mathbf{k},M}) &= \int_{[0,1]^d} m(\mathbf{z}) \log \left( \frac{b_{\mathbf{k},M}(\mathbf{z})}{m(\mathbf{z})} \right) d\mathbf{z}, \\ &= \int_{R_1} m(\mathbf{z}) \log \left( \frac{b_{\mathbf{k},M}(\mathbf{z})}{m(\mathbf{z})} \right) d\mathbf{z} + \int_{R_2} m(\mathbf{z}) \log \left( \frac{b_{\mathbf{k},M}(\mathbf{z})}{m(\mathbf{z})} \right) d\mathbf{z} \\ &\quad + \int_{R_3} m(\mathbf{z}) \log \left( \frac{b_{\mathbf{k},M}(\mathbf{z})}{m(\mathbf{z})} \right) d\mathbf{z}. \end{aligned}$$

The first of these summands can be made smaller than an arbitrary target  $\delta_1$  as follows: Observe that since  $m$  is continuous on a compact domain, it is bounded above by a number  $\mu$  such that  $m(\mathbf{z}) < \mu$  for all  $\mathbf{z} \in R_1$ . Since  $\log$  is uniformly continuous on  $[\beta, \infty)$ , there is an  $\epsilon_1$  such that if  $|a - b| < \epsilon_1$  then  $\log\left(\frac{a}{b}\right) = \log(a) - \log(b) \leq |\log(a) - \log(b)| < \frac{\delta_1}{\mu}$ . Since  $b_{\mathbf{k},M}(\mathbf{z})$  approaches  $m(\mathbf{z})$  uniformly over  $R_1$ , there is a non-negative integer  $\lambda$  such that  $|b_{\kappa,M}(\mathbf{x}) - m(\mathbf{x})| < \epsilon_1$  for all  $\mathbf{x}$  in  $R_1$  for all and for all  $\kappa \in \mathbb{N}^d$ , such that  $\kappa_i > \lambda$ ,  $i = 1, \dots, d$ . Pick  $\mathbf{l}$  such that  $p_k(\mathbf{l}) > 0$  and each  $l_i > \lambda$ . Then, it follows that

$$\int_{R_1} m(\mathbf{z}) \log \left( \frac{b_{\mathbf{l},M}(\mathbf{z})}{m(\mathbf{z})} \right) d\mathbf{z} \leq \int_{R_1} \mu \frac{\delta_1}{\mu} \leq \delta_1.$$

The second summand can be made smaller than a target  $\delta_2$  by observing that since  $M$  has finite entropy (from condition (i)), it is possible to reduce  $R_2$  to an area where  $\int_{R_2} m(\mathbf{z}) \log(m(\mathbf{z})) d\mathbf{z} < \delta_2$ . We now observe that in all of  $R_2$ ,  $m(\mathbf{z}) > 1$ , so  $\log\left(\frac{b_{\mathbf{l},M}(\mathbf{z})}{m(\mathbf{z})}\right) < \log(b_{\mathbf{l},M}(\mathbf{z}))$ . Hence, it follows that

$$\int_{R_2} m(\mathbf{z}) \log \left( \frac{b_{\mathbf{l},M}(\mathbf{z})}{m(\mathbf{z})} \right) d\mathbf{z} < \delta_2.$$

Lastly, to show that the third summand can be made smaller than a target  $\delta_3$ , We observe that in  $R_3$ ,  $\beta < m(\mathbf{z}) < \mu$  and  $\beta < b_{\mathbf{l},M}(\mathbf{z}) < \mu$ . We set the measure of this region to be smaller than  $\frac{\delta_3}{\mu \log(\mu/\beta)}$  and we have

$$\int_{R_3} m(\mathbf{z}) \log \left( \frac{b_{1,M}(\mathbf{z})}{m(\mathbf{z})} \right) d\mathbf{z} \leq \int_{R_3} \mu \frac{\delta_3}{\mu} \leq \delta_3.$$

Pick  $\delta_1 = \delta_2 = \delta_3 = \epsilon/6$  and select  $\mathbf{l}$  accordingly. We now have that  $\mathcal{KL}(M, B_{\mathbf{l},M}) \leq \frac{\epsilon}{2}$ .

By Proposition 1, there is a unique yett-uniform copula  $C^{(0)}$  such that  $T_{[0,1]^d} \circ BP_{(\rho^{\mathbf{l}}, C^{(0)})} = B_{\mathbf{l},M}$ . By Theorem 4, there is an open Kullback–Leibler neighborhood of  $C^{(0)}$ ,  $A_\epsilon^{C^{(0)}}$  such that if  $C \in \{T_{[0,1]} \circ BP_{(\rho^{\mathbf{l}}, G)} : G \in A_\epsilon^{C^{(0)}}\}$ , then  $\mathcal{KL}(C, B_{\mathbf{l},M}) < \frac{\epsilon}{2}$ .

In Lemma 2 of the Supplementary Material of Kuschinski and Jara (2023), they showed that open sets in both the Hellinger and Kullback–Leibler sense have positive probability under the prior  $p(\cdot \mid \mathbf{k}, \alpha, G_0)$ , for any  $\mathbf{k} \in \mathbb{N}^d$ . Hence,

$$p(\{T_{[0,1]} \circ BP_{(\rho^{\mathbf{k}}, G)} : G \in A_\epsilon^{C^{(0)}}\} \mid \mathbf{l}, \alpha, G_0) > 0.$$

Observe that  $\{T_{[0,1]} \circ BP_{(\rho^{\mathbf{k}}, G)} : G \in A_\epsilon^{C^{(0)}}\} \subseteq A_\epsilon^M$  so

$$\Pi(A_\epsilon^M \mid \alpha, G_0, p_{\mathbf{k}}) \geq p(\{T_{[0,1]} \circ BP_{(\rho^{\mathbf{k}}, G)} : G \in A_\epsilon^{C^{(0)}}\} \mid \mathbf{l}, \alpha, G_0) > 0,$$

which completes the proof. □

## 8 Proof of Theorem 7

Consider a Kullback-Leibler neighborhood  $\mathcal{K}$  which contains the copula  $M$ . Then there is an  $\epsilon > 0$  such that

$$\mathcal{K}^* = \{Q \in \mathcal{C}_d : \mathcal{KL}(Q||M) < \epsilon\} \subseteq \mathcal{K}.$$

By Theorem 6, it follows that  $\Pi(\mathcal{K}^*) > 0$ . We note that  $\Pi(\mathcal{K}) \geq \Pi(\mathcal{K}^*) > 0$  so  $M$  is in the Kullback-Leibler support of the prior. Hence, it follows by Schwartz's theorem (Schwartz, 1965) that for every weak neighborhood  $A^M$  of  $M$  we have

$$\Pi(A^M | \alpha, G_0, p_{\mathbf{k}}, \mathbf{x}_1, \dots, \mathbf{x}_n) \xrightarrow[n \rightarrow +\infty]{} 1,$$

$P$ - almost surely, which completes the proof. □

## 9 Proof of Theorem 8

We note that  $\pi(\cdot \mid \alpha, G_0, p_k)$  is a mixture of the form

$$\pi(\cdot \mid \alpha, G_0, p_k) = \sum_{r=1}^{\infty} p_k(r) \pi(\cdot \mid r, \alpha, G_0),$$

where  $\pi(\cdot \mid r, \alpha, G_0)$  is the density of  $BYUP(\mathbf{k}, \alpha, G_0)$ , where  $\mathbf{k}$  is such that  $r = k_1 = \dots = k_d$ . Now, let  $I_r(\delta)$  be the number of Hellinger balls of radius  $\delta$  required to cover the space  $\mathcal{BC}_{d,\mathbf{k}}$ , where  $\mathbf{k}$  is such that  $r = k_1 = \dots = k_d$ . Let  $C^{(1)}$  and  $C^{(2)}$  be two Bernstein yett-uniform copulas of degree  $r$ , with densities  $c^{(1)}$  and  $c^{(2)}$ , and weights  $\mathbf{W}^{(1)}$  and  $\mathbf{W}^{(2)}$ , respectively. The squared Hellinger distance between  $C^{(1)}$  and  $C^{(2)}$ , is given by

$$\begin{aligned} \mathcal{H}^2(C^{(1)}, C^{(2)}) &= \frac{1}{2} \int_{[0,1]^d} \left( \sqrt{c^{(1)}(\mathbf{z})} - \sqrt{c^{(2)}(\mathbf{z})} \right)^2 d\mathbf{z}, \\ &= \frac{1}{2} \int_{[0,1]^d} \left( \sqrt{\sum_{v_1=1}^r \dots \sum_{v_d=1}^r W_{\nu_1, \dots, \nu_d}^{(1)} \prod_{j=1}^d \beta(z_j \mid \nu_j, r - \nu_j + 1)} \right. \\ &\quad \left. - \sqrt{\sum_{v_1=1}^r \dots \sum_{v_d=1}^r W_{\nu_1, \dots, \nu_d}^{(2)} \prod_{j=1}^d \beta(z_j \mid \nu_j, r - \nu_j + 1)} \right)^2 d\mathbf{z}, \\ &\leq \left( \sqrt{\sum_{v_1=1}^r \dots \sum_{v_d=1}^r W_{\nu_1, \dots, \nu_d}^{(1)}} - \sqrt{\sum_{v_1=1}^r \dots \sum_{v_d=1}^r W_{\nu_1, \dots, \nu_d}^{(2)}} \right)^2, \\ &\leq \sum_{v_1=1}^r \dots \sum_{v_d=1}^r \left( \sqrt{W_{\nu_1, \dots, \nu_d}^{(1)}} - \sqrt{W_{\nu_1, \dots, \nu_d}^{(2)}} \right)^2. \end{aligned}$$

Let  $\sqrt{\mathbf{W}^{(1)}}$  and  $\sqrt{\mathbf{W}^{(2)}}$  be the vectors of the element-wise square roots the vectors  $\mathbf{W}^{(1)}$  and  $\mathbf{W}^{(2)}$  respectively. Observe that the last expression is the square of the Euclidean distance between these vectors. Hence  $\mathcal{H}(C^{(1)}, C^{(2)}) \leq \left\| \sqrt{\mathbf{W}^{(1)}} - \sqrt{\mathbf{W}^{(2)}} \right\|$ , where  $\|\cdot\|$  is the Euclidean norm. In other words, if a Euclidean ball of radius  $\delta$  includes  $\sqrt{\mathbf{W}^{(1)}}$  and  $\sqrt{\mathbf{W}^{(2)}}$ , then  $C^{(1)}$  and  $C^{(2)}$  are in a corresponding Hellinger ball of radius  $\delta$  also. As a result,  $I_r(\delta)$  is at most the number of Euclidean balls required to cover the space of possible weights for BYU copulas of degree  $r$ .

Note that every element of  $\sqrt{\mathbf{W}^{(i)}}$  is between 0 and  $1/\sqrt{r}$ . The length of these vectors is  $r^d$ , so the space of possible weights is contained in  $[0, 1/\sqrt{r}]^{r^d}$ . Consider covering this box with Euclidean balls of radius  $\delta$ . There is an  $\epsilon$  such that it takes at most  $\left(\frac{\epsilon}{\delta\sqrt{r}}\right)^{r^d}$  of them. As such, we observe that  $I_r(\delta) \leq \left(\frac{\epsilon}{\delta\sqrt{r}}\right)^{r^d}$ .

Let  $M \in \tilde{C}_d$ . From Theorem 6 we know that  $M$  is in the Kullback-Leibler support of the prior. Now assume that  $\bar{P}_l < p^{l^d+a}$  for some  $0 < p < 1$ , some  $\alpha$ , and large enough  $l$ . Then, by the result of Xing and Ranneby (2012), (Section 6.3), we have that

$$\Pi(A_\epsilon^M \mid \alpha, G_0, \mathbf{x}_1, \dots, \mathbf{x}_k) \xrightarrow{n \rightarrow +\infty} 1,$$

for all  $\epsilon > 0$ , which completes the proof.  $\square$

## 10 Sampling a yett-uniform copula polytope vertex

For a given  $d$  and  $\mathbf{k}$ , the polytope of the yett-uniform copulas for those parameters is defined. Thus the input to randomly sampling a vertex of that space requires only  $d$  and  $\mathbf{k}$ . The vertices are the most extreme points in the polytope, in other words, the vertices will have the most cells equal to zero as possible for any yett-uniform copula in that space. Once one vertex is found the others are just permutations of the indices in each dimension. An algorithm to select a random vertex, for the case of  $k_i = k_j$  for all  $i$  and  $j$  in  $\{1, \dots, d\}$ , is given in Algorithm 1.

---

**Algorithm 1:** Algorithm to sample a vertex from a yett-uniform copula

---

**Input:**  $d$  and  $\mathbf{k}$ , with  $k_i = k_j$  for all  $i$  and  $j$  in  $\{1, \dots, d\}$ .

**Step 1:** Construct  $E$ , a  $d$ -dimensional yett defined by  $\mathbf{k}$  with no assigned probability;

**Step 2:** Assign mass of  $1/k_1$  to each diagonal element (i.e., the cells with equal indices in all dimensions);

**Step 3:** Randomly permute the indices of  $E$  in each dimension;

**Output:**  $E$ , a random vertex from the copula polytope.

---

A simple two dimensional illustration follows. The inputs are  $d = 2$ ,  $\mathbf{k} = (4, 4)$ . In Step 1 we have

$$E = \begin{bmatrix} 0 & | & 0 & | & 0 & | & 0 \\ 0 & | & 0 & | & 0 & | & 0 \\ 0 & | & 0 & | & 0 & | & 0 \\ 0 & | & 0 & | & 0 & | & 0 \end{bmatrix}.$$

Next in Step 2 we set the diagonal elements of the array to be equal to  $1/k_1 = 1/4$ .

$$E = \begin{bmatrix} 1/4 & | & 0 & | & 0 & | & 0 \\ 0 & | & 1/4 & | & 0 & | & 0 \\ 0 & | & 0 & | & 1/4 & | & 0 \\ 0 & | & 0 & | & 0 & | & 1/4 \end{bmatrix}.$$

Next we randomly permute the indices in the first dimension and, for one realization, get

$$E = \begin{bmatrix} 1/4 & | & 0 & | & 0 & | & 0 \\ 0 & | & 0 & | & 1/4 & | & 0 \\ 0 & | & 1/4 & | & 0 & | & 0 \\ 0 & | & 0 & | & 0 & | & 1/4 \end{bmatrix}.$$

To finish Step 3 we randomly permute the indices in the second dimension and, for one realization, get

$$E = \begin{bmatrix} 0 & | & 0 & | & 1/4 & | & 0 \\ 1/4 & | & 0 & | & 0 & | & 0 \\ 0 & | & 0 & | & 0 & | & 1/4 \\ 0 & | & 1/4 & | & 0 & | & 0 \end{bmatrix}.$$

This is the resulting uniformly sampled vertex,  $E$ , of the algorithm.

## 11 Additional details for two proposal schemes

We add some additional details about the generalized rectangular exchange and the vertex-line proposals in this section. In both proposals a line segment is defined which contains all possible proposals.

### 11.1 The generalized rectangular exchange proposal

For this proposal there are a couple of minor points to consider. First, in the reserve step it is possible that both the same  $Z_1$  and  $Z_2$  are selected but in the opposite order. In this case there are two possible ways that could produce the chain with a current location of  $G^*$  with a proposal of  $G^{(i)}$ . However, both orders are also possible in the forward case and any adjustment needed in the Hastings ratio cancels.

The other consideration is if  $Z_1 = Z_2$ . We define this case to just have the proposal  $G^* = G^{(i)}$ . Therefore regardless of the decision to accept or reject the proposal, it would produce the same value for  $G^{(i+1)}$ , and only impact the acceptance rate.

### 11.2 The vertex-line proposal

There are a couple other subtleties that we address here. First, for this proposal it is possible that the far boundary is also a vertex. The probability of this is minuscule, however, if this occurs, it has possible implications for the reversibility condition. In this case there are two possible vertices that could produce the chain with a current location of  $G^*$  with a proposal of  $G^{(i)}$ . However, both of these vertices are also possible in the forward case and any adjustment needed in the Hastings ratio cancels.

The other consideration is if the current state,  $G^{(i)}$ , is a vertex. Typically, the algorithm would proceed as normal, but in the rare case that the selected vertex  $E$  (in Step 1 of Algorithm 3) is equal to  $G^{(i)}$ , then the proposal would by definition be  $G^{(i)}$ . Therefore regardless of the decision to accept or reject the proposal, it would produce the same value for  $G^{(i+1)}$ , and only impact the acceptance rate.

## References

- Ash, J. M. (2008). Mean value theorems for differences. *Elemente der Mathematik*, 63(3):122–125.
- Barrientos, A. F., Jara, A., and Quintana, F. A. (2015). Bayesian density estimation for compositional data using random Bernstein polynomials. *Journal of Statistical Planning and Inference*, 166:116–125.
- Boole, G. (1854). *An Investigation of the Laws of Thought on Which are Founded the Mathematical Theories of Logic and Probabilities*. Walton and Maberly, London.
- Courant, R. (1950). *Differential and integral calculus. Vol. II*. Interscience Publishers, Inc., New York. Translated from the German by E. J. McShane, Reprint of the second edition (1937), A Wiley-Interscience Publication.
- Kuschinski, N. and Jara, A. (2023). Grid-uniform copulas and rectangle exchanges: Bayesian model and inference for a rich class of copula functions. *Bayesian Analysis*, pages 1 – 28.
- Sancetta, A. and Satchell, S. (2004). The Bernstein copula and its applications to modeling and approximations of multivariate distributions. *Econometric Theory*, 20(3):535–562.
- Schwartz, L. (1965). On Bayes procedures. *Z. Wahrscheinlichkeitstheorie verw Gebiete*, 4(1):10–26.
- Xing, Y. and Ranneby, B. (2012). On strong Hellinger consistency of posterior distributions. *Journal of Nonparametric Statistics*, 24(2):505–515.
